# Supplementary material for: Improving Diversity in Black-box Few-shot Knowledge Distillation
Source: arXiv:2604.25795 source file (2026-04-28)
Supplement: Supplementary file 1 [file supp-standalone.tex]

\documentclass[12pt]{article}

% Import preamble
\input{./preamble.tex}

% Paper-specific settings
\title{[Supplementary Material] \\ Improving Diversity in \\ Black-box Few-shot Knowledge Distillation}
\author[1]{Tri-Nhan Vo}
\author[1]{Dang Nguyen}
\author[1]{Kien Do}
\author[1]{Sunil Gupta}
\affil[1]{Applied Artificial Intelligence Institute (A2I2), Deakin University, Australia}
\affil[1]{\texttt{\{s223032975, d.nguyen, k.do, sunil.gupta\}@deakin.edu.au}}
\runningheads{T-N. Vo et al.}{Supplementary Material: DivBFKD}
\date{\small{Accepted at ECML-PKDD 2024}}

\begin{document}

\maketitle

\input{./supp.tex}

\bibliography{references}

\end{document}
